# Supplementary material for: AxonEM Dataset: 3D Axon Instance Segmentation of Brain Cortical Regions
Source: arXiv:2107.05451 source file (2021-07-12)
Supplement: Supplementary file 1 [file supplement.tex]

\newpage
\title{\small{Supplementary Materials on:}\\\Large{MitoEM Dataset: Large-scale 3D Mitochondria Instance Segmentation from EM Images}}
\titlerunning{MitoEM Dataset}

\newcommand*{\affaddr}[1]{#1} % No op here. Customize it for different styles.
\newcommand*{\affmark}[1][*]{\textsuperscript{#1}}

\author{Donglai Wei\affmark[1] \and Zudi Lin\affmark[1] \and Nils Wendt\affmark[2]\thanks{\footnotesize Works are done during internship at Harvard Univeristy} \and Xingyu Liu\affmark[3$\star$] \and Aarush Gupta\affmark[4$\star$] \and Daniel Franco-Barranco\affmark[5,6] \and Wenjie Yin\affmark[1$\star$]  \and Xin Huang\affmark[8$\star$]  \and Won-Dong Jang\affmark[1] \and Xueying Wang\affmark[1] \and Ignacio Arganda-Carreras\affmark[5,6,7] \and Jeff W. Lichtman\affmark[1] \and Hanspeter Pfister\affmark[1]}
\authorrunning{D. Wei {\em et al.}}
%\author{Submission ID 239}
%\authorrunning{Submission ID 239}
\institute{
\affaddr{\affmark[1] Harvard University} \
\affaddr{\affmark[2] Technical University of Munich} \
\affaddr{\affmark[3] Shanghai Jiao Tong University } \
\affaddr{\affmark[4] Indian Institute of Technology Roorkee} \
\affaddr{\affmark[5] Donostia International Physics Center (DIPC)} \
\affaddr{\affmark[6] University of the Basque Country} \
\affaddr{\affmark[7] Ikerbasque, Basque Foundation for Science (UPV/EHU)} \
\affaddr{\affmark[8] Northeastern University}\\
\email{donglai@seas.harvard.edu}
}
\maketitle

\beginsupplement
%\vspace{-0.1in}
\begin{table}[ht]
\caption{Hyper-parameter selection. We find the best hyper-parameters for decoding approaches on MitoEM-H validation sets and apply them for MitoEM test sets (human and rat) in the main paper. Specifically, three parameters are the thresholds for semantic map ($\alpha$), seed map ($\beta$), and contour map ($\gamma$).}
\vspace{0.1in}
\centering
\resizebox{\textwidth}{!}{
\begin{tabular}{lllccccc}
\hline
\multicolumn{2}{l}{\multirow{2}{*}{Method}}&
\multicolumn{1}{l}{\multirow{2}{*}{Parameter(s)}}&
\multicolumn{4}{c}{AP-75} & 
~\multirow{2}{*}{$\#$ Instances}
\\\cline{4-7}
& & &~Small~ & ~Med~ & ~Large~ &~All~ & \\
\hline
%$\alpha$=0.25 & 0.234 & 0.539 & 0.469 & 0.330 & 3181\\
    \multirow{6}{*}{U3D-B}&
    \multirow{6}{*}{~+CC~}&
    $\alpha$=0.50 & 0.426 & 0.673 & 0.537 & 0.482 & 2582\\
    & & $\alpha$=0.75 & 0.498 & 0.735 & 0.571 & 0.545 & 2426\\
    & & $\alpha$=0.85 & 0.491 & 0.742 & 0.566 & 0.550 & 2344\\
    & & $\alpha$={\bf 0.90} & 0.484 & 0.742 & 0.565 & {\bf 0.552} & 2298\\
    & & $\alpha$=0.95 & 0.444 & 0.746 & 0.579 & 0.542 & 2224\\
    \hline
    \multirow{3}{*}{U3D-B}&
    \multirow{3}{*}{~+MW~}&
    ($\alpha$,$\beta$)=(0.90,0.93) & 0.492 & 0.757 & 0.575 & 0.566 & 2425\\
    & & ($\alpha$,$\beta$)=(0.90,0.95) & 0.493 & 0.768 & 0.579 & 0.577 & 2740\\
    & & ($\alpha$,$\beta$)=({\bf 0.90,0.98}) & 0.488 & 0.790 & 0.625 & {\bf 0.592} & 3117\\
    \hline
    \multirow{3}{*}{U3D-BC}&
    \multirow{3}{*}{~+CC~}&
    ($\alpha$,$\gamma$)=(0.90,0.98) & 0.483 & 0.771 & 0.608 & 0.570 & 2434 \\
    & & ($\alpha$,$\gamma$)=(0.90,0.95) & 0.519 & 0.802 & 0.655 & 0.614 & 2487\\
    & & ($\alpha$,$\gamma$)=({\bf 0.90,0.90}) & 0.523 & 0.833 & 0.636 & {\bf 0.623} & 2574\\
    \hline
    \multirow{3}{*}{U3D-BC}&
    \multirow{3}{*}{~+MW~}&
    ($\alpha$,$\beta$,$\gamma$)=(0.90,0.98,0.95) & 0.490 & 0.801 & 0.625 & 0.596 & 3173\\
    & & ($\alpha$,$\beta$,$\gamma$)=(0.90,0.95,0.95) & 0.517 & 0.803 & 0.637 & 0.613 & 2803\\
    & & ($\alpha$,$\beta$,$\gamma$)=({\bf 0.90,0.95,0.90}) & 0.523 & 0.829 & 0.633 & {\bf 0.624} & 2900\\
    \hline
\end{tabular}}
\end{table}

\begin{figure}[ht]
     \centering
     \includegraphics[width=0.9\textwidth]{figures/result/result_lucchi.pdf}
     \caption{Comparison on the Lucchi dataset. (b) FFN cannot capture the instance geometry well. (c) U3D-BC+MW only misses small instances on the border.}
     \label{fig:dataset_stat}
\end{figure}

% \begin{figure}[t]
%      \centering
%      \begin{minipage}[b]{\linewidth}
%      \centering
%      \includegraphics[width=0.7\textwidth]{figures/supp/supp_f1.pdf}
%      \subcaption{}
%      \end{minipage}
%      \begin{minipage}[b]{\linewidth}
%      \centering
%      \includegraphics[width=0.8\textwidth]{figures/supp/supp_f2.pdf}
%      \subcaption{}
%      \end{minipage}
%      \begin{minipage}[b]{\linewidth}
%      \centering
%      \includegraphics[width=0.7\textwidth]{figures/supp/supp_f3.pdf}
%      \subcaption{}
%      \end{minipage}
%      \caption{Visualization of MitoEM Dataset. (a) We show the scatter plots for all mitochondria in MitoEM. For each mitochondrion, the $x$-axis is the number of skeleton vertices, approximating its length, and the $y$-axis is its volume. We fit a line on the 2D plot for each tissue and sample examples along each line with increasing number of skeleton vertices ($\textcircled{\raisebox{-0.9pt}{1}}$-\textcircled{\raisebox{-0.9pt}{7}}). (b) Mitochondria from two tissues have similar topology, where ones from MitoEM-H have thin connections. (c) We show some extra-large mitochondria instances that are out of the plot (a).}
%      \label{fig:dataset_stat}
% \end{figure}

\begin{figure}[t]
     \centering
     \begin{minipage}[b]{\linewidth}
     \centering
     \includegraphics[width=0.7\textwidth]{figures/supp/supp_f3.pdf}
     \subcaption{}
     \end{minipage}
     \caption{Visualization of extra-large mitochondria instances in the MitoEM Dataset.}
     \label{fig:dataset_stat}
\end{figure}
